# Supplementary material for: A Model for Multi-Agent Heterogeneous Interaction Problems
Source: arXiv:2208.01430 source file (2024-09-19)
Supplement: Supplementary file 1 [file appendix.tex]

% !TEX root = ./root.tex

\section{Appendix}
\label{s:appendix}

The optimal defender distribution $P_d^*$ is found by minimizing~\cref{eq:harm} with respect to $P_d$, subject to constraints of non-negativity ($P_d \geq 0$) and normalization ($\sum_d P_d = 1$). We can define an augmented Lagrangian as
\[
    L = \sum_a Q_a \Bar{F}_a + \l \rbr{\sum_d P_d - 1} - \sum_d \nu_d P_d
\]
where $\l$ and $\nu_d$ are Largrange multipliers and set its derivative to zero to get the optimality conditions
\[
    \aed{
    \sum_a Q_a \Tilde{P}_a^{-\a}\ \G(1+\alpha) &= -\l^* + \nu_d^*\\
    \nu_d^* &\geq 0 \qquad \text{(dual feasibility)}\\
    \nu_d^* P_d^* &= 0 \qquad \text{(complementary slackness)}
}
\]
If $P_d^* > 0$ for some $d$, we have $\nu_d^* = 0$ and thus $\sum_a Q_a\ \Tilde{P}_a^{-\a}\ \G(1+\alpha) = -\l^*$. We can solve these equations for specific choices of cross-reactivity $f_{d,a}$~\cite{Mayer_organized}.

If the shape-space is continuous and the cross-reactivity is $f_{d,a} = f(d-a)$, then we can write the first condition as
\[
    \int \dd{a} Q_a \Bar{F}'(\tilde{P}^*_a) f(d-a) = -\l^*
\]
where the total probability of tackling attacker $a$ is again a convolution $\tilde{P}^*_a = \int \dd{d} P_d f(d-a)$. We can now solve for $\tilde{P}^*_a$ by noticing that $Q_a \Bar{F}'(\tilde{P}^*_a) f(d-a) = -c$ satisfies this equation for some constant $c$ (the convolution of a constant is a constant). Given such a $\tilde{P}^*$ we can calculate the optimal defender distribution as
\[
    P_d^* = \FF^{-1}[\FF[\tilde{P}^*]/\FF[f] ].
\]
where $\FF[\cdot]$ denotes the Fourier transform~\cite{Mayer_organized}.
